# Supplementary material for: Open-Shell Coupled-Cluster Valence-Bond Theory Augmented with an Independent Amplitude Approximation for Three-Pair Correlations: Application to a Model Oxygen-Evolving Complex and Single Molecular Magnet
Source: arXiv:1808.06743 source file (2018-12-31)
Supplement: Supplementary file 1 [file supporting_information.pdf]

# Supplementary Material: Open-Shell Coupled-Cluster Valence-Bond Theory Augmented with an Independent Amplitude Approximation for Three-Pair Correlations: Application to a Model Oxygen-Evolving Complex and Single Molecular Magnet

Joonho Lee,* David W. Small,* and Martin Head-Gordon*

*Department of Chemistry, University of California, Berkeley, California 94720, USA*

*Chemical Sciences Division, Lawrence Berkeley National Laboratory, Berkeley, California 94720, USA*

E-mail: linusjoonho@gmail.com; dsmallchem@gmail.com; mhg@cchem.berkeley.edu

## Definitions

We begin by defining some fundamental quantities that will be used to compute matrix elements and other relevant quantities discussed in the main text. Many of definitions below are already given in ref. 61, but it is our intention to keep this paper as self-contained as possible. Interested readers shall refer to 61 although it is not necessary unless otherwise noted.

We define a set of spin orbitals $S_a$ for a pair $a$,

$$S_a = \{a_\alpha, a_\beta, \hat{a}_\alpha, \hat{a}_\beta\} \tag{S1}$$

We define the density matrix of a closed-shell pair $K$,

$$P_{K;wx;pr} = \langle 0| \, g_{w,K} a_p^\dagger a_r g_{x,K}^\dagger \, |0\rangle \tag{S2}$$

where $w$ and $x$ denote the spin states of the pair either $s, t_1, t_2$, or $t_3$ and $p$ and $r$ denotes the spin-orbital indices in the set $S_K$. For a singly occupied orbital (or an open-shell pair) $\mu$, only $P_{\mu;ss;\mu_\alpha\mu_\alpha} = 1$ and all the other elements are zero as they include the fictitious orbital. These are used to define the following quantities: the one-body contribution reads

$$\eta_{a;wx} = \sum_{pr \in S_a} h_{pr} P_{K;wx;pr}, \tag{S3}$$

and the intrageminal Coulomb contribution follows

$$\rho_{a;w;x} = \sum_{prqs \in S_a} \langle pq||rs\rangle \, f_{a;w;pq} f_{a;x;rs}, \tag{S4}$$

and the intergeminal Coulomb contribution reads

$$\sigma_{ab;wx;yz} = \sum_{pr \in S_a} \sum_{qs \in S_b} \langle pq||rs\rangle \, P_{a;wx;pr} P_{b;yz;qs}, \tag{S5}$$

where

$$f_{K;s;K_\alpha K_\beta} = \frac{2\cos(\theta_K)}{\sqrt{2(1+\cos^2(\theta_K))}}, \tag{S6}$$

$$f_{K;s;K_\alpha \hat{K}_\beta} = f_{K;s;\hat{K}_\alpha K_\beta} = \frac{-\sin(\theta_K)}{\sqrt{2(1+\cos^2(\theta_K))}} \tag{S7}$$

$$f_{K;t_1;K_\alpha \hat{K}_\beta} = -f_{K;t_1;\hat{K}_\alpha K_\beta} = -f_{K;t_2;K_\alpha \hat{K}_\alpha} = -f_{K;t_2;K_\beta \hat{K}_\beta} = -\frac{1}{\sqrt{2}} \tag{S8}$$

and all the other $f$'s are zero. Obviously, we have $\rho_{\mu;w;x} = 0$.

## **Proof of Eq.** (40)

In the main text, we proved that if $b$ is not on the same fragment as $K$ then the size-consistency claim is satisfied as $t_{Kb} = 0$. The rest of the proof is then showing that the following matrix element is zero when $b$ is on the same fragment as $K$:

$$\begin{aligned} \langle \Psi_{(KLa)} | \hat{\mathcal{H}} | \Phi_{(Kb)(La)} \rangle = & -\frac{3}{10} \langle \Psi_{(KLa)} | \hat{\mathcal{H}} | \Psi_{(KL)(ab)} \rangle - \frac{3}{10} \langle \Psi_{(KLa)} | \hat{\mathcal{H}} | \Psi_{(Ka)(Lb)} \rangle \\ & + \frac{6}{5} \langle \Psi_{(KLa)} | \hat{\mathcal{H}} | \Psi_{(Kb)(La)} \rangle \end{aligned} \tag{S9}$$

where we wrote $|\Phi_{(Kb)(La)}\rangle$ in terms of $|\Psi_{(KL)(ab)}\rangle$, $|\Psi_{(Ka)(Lb)}\rangle$, and $|\Psi_{(Kb)(La)}\rangle$ using the relevant $\mathbf{S}^+$ in this 8-electron singlet subspace (see ref. 48 for details). After some algebra, one can show that

$$\langle \Psi_{(KLa)} | \hat{\mathcal{H}} | \Phi_{(Kb)(La)} \rangle = \frac{3\sqrt{6}}{10} \left( \sigma_{Kb;t_1t_3;st_2} + \sigma_{Kb;t_1t_2;st_3} \right) + \frac{2}{5} \langle \Psi_{[K]_1[L]_2[a]_3} | \hat{\mathcal{H}} | \Psi_{[K]_1[b]_1[L]_2[a]_3} \rangle = 0 \tag{S10}$$

The first term is zero because $\sigma_{Kb;t_1t_3;st_2} = -\sigma_{Kb;t_1t_2;st_3}$ and it can be shown that the second term is also zero after little more algebra. Therefore, we proved Eq. (40).

## S and $\mathbf{S}^+$ within the five-pair substitutions

The overlap matrix among vectors in the dual frame within the five-pair (5P) substitutions is

$$\mathbf{S}_{5\mathrm{P}} = \begin{bmatrix} 1 & \frac{1}{3} & -\frac{1}{3} & \frac{1}{3} & \frac{1}{3} & -\frac{1}{3} & \frac{1}{3} & 0 & 0 & 0 \\ \frac{1}{3} & 1 & 0 & 0 & -\frac{1}{3} & \frac{1}{3} & 1 & 0 & \frac{1}{3} & -\frac{1}{3} \\ -\frac{1}{3} & 0 & 1 & \frac{1}{3} & 0 & \frac{1}{3} & 0 & -\frac{1}{3} & 0 & \frac{1}{3} \\ \frac{1}{3} & 0 & \frac{1}{3} & 1 & \frac{1}{3} & 0 & 0 & -\frac{1}{3} & \frac{1}{3} & 0 \\ \frac{1}{3} & -\frac{1}{3} & 0 & \frac{1}{3} & 1 & \frac{1}{3} & -\frac{1}{3} & \frac{1}{3} & -\frac{1}{3} & 0 \\ -\frac{1}{3} & \frac{1}{3} & \frac{1}{3} & 0 & \frac{1}{3} & 1 & \frac{1}{3} & \frac{1}{3} & 0 & -\frac{1}{3} \\ \frac{1}{3} & 1 & 0 & 0 & -\frac{1}{3} & \frac{1}{3} & 1 & 0 & \frac{1}{3} & -\frac{1}{3} \\ 0 & 0 & -\frac{1}{3} & -\frac{1}{3} & \frac{1}{3} & \frac{1}{3} & 0 & 1 & \frac{1}{3} & \frac{1}{3} \\ 0 & \frac{1}{3} & 0 & \frac{1}{3} & -\frac{1}{3} & 0 & \frac{1}{3} & \frac{1}{3} & 1 & \frac{1}{3} \\ 0 & -\frac{1}{3} & \frac{1}{3} & 0 & 0 & -\frac{1}{3} & -\frac{1}{3} & \frac{1}{3} & \frac{1}{3} & 1 \end{bmatrix} \tag{S11}$$

where we ordered columns and rows as $|\Psi_{(bc)(KLa)}\rangle$, $|\Psi_{(ab)(KLc)}\rangle$,$|\Psi_{(Lb)(Kac)}\rangle$, $|\Psi_{(Kb)(Lac)}\rangle$, $|\Psi_{(Kc)(Lab)}\rangle$, $|\Psi_{(Lc)(Kab)}\rangle$, $|\Psi_{(ac)(KLb)}\rangle$, $|\Psi_{(KL)(abc)}\rangle$, $|\Psi_{(Ka)(Lbc)}\rangle$, and $|\Psi_{(La)(Kbc)}\rangle$. As we expect only six orthogonal singlet configurations in this 12-electron singlet space, these 10 vectors are necessarily linearly-dependent. Indeed, there are 4 zero singular values along with 6 non-zero singular values, $\frac{1}{3}(5 \pm 2\sqrt{2})$ and four $\frac{5}{3}$'s. The corresponding pseudoinverse

is then

$$
\mathbf{S}^{+}_{5\mathrm{P}} = \begin{bmatrix}
\frac{681}{1445} & \frac{39}{289} & \frac{57}{1445} & \frac{-57}{1445} & \frac{243}{1445} & \frac{-243}{1445} & \frac{39}{289} & 0 & \frac{-60}{289} & \frac{60}{289} \\
\frac{39}{289} & \frac{57}{289} & \frac{30}{289} & \frac{-30}{289} & \frac{-9}{289} & \frac{9}{289} & \frac{57}{289} & 0 & \frac{-21}{289} & \frac{21}{289} \\
\frac{57}{1445} & \frac{30}{289} & \frac{3954}{7225} & \frac{-486}{7225} & \frac{201}{7225} & \frac{666}{7225} & \frac{30}{289} & \frac{-3}{25} & \frac{-1554}{7225} & \frac{2421}{7225} \\
\frac{-57}{1445} & \frac{-30}{289} & \frac{-486}{7225} & \frac{3954}{7225} & \frac{666}{7225} & \frac{201}{7225} & \frac{-30}{289} & \frac{-3}{25} & \frac{2421}{7225} & \frac{-1554}{7225} \\
\frac{243}{1445} & \frac{-9}{289} & \frac{201}{7225} & \frac{666}{7225} & \frac{2454}{7225} & \frac{1014}{7225} & \frac{-9}{289} & \frac{3}{25} & \frac{-921}{7225} & \frac{54}{7225} \\
\frac{-243}{1445} & \frac{9}{289} & \frac{666}{7225} & \frac{201}{7225} & \frac{1014}{7225} & \frac{2454}{7225} & \frac{9}{289} & \frac{3}{25} & \frac{54}{7225} & \frac{-921}{7225} \\
\frac{39}{289} & \frac{57}{289} & \frac{30}{289} & \frac{-30}{289} & \frac{-9}{289} & \frac{9}{289} & \frac{57}{289} & 0 & \frac{-21}{289} & \frac{21}{289} \\
0 & 0 & \frac{-3}{25} & \frac{-3}{25} & \frac{3}{25} & \frac{3}{25} & 0 & \frac{9}{25} & \frac{3}{25} & \frac{3}{25} \\
\frac{-60}{289} & \frac{-21}{289} & \frac{-1554}{7225} & \frac{2421}{7225} & \frac{-921}{7225} & \frac{54}{7225} & \frac{-21}{289} & \frac{3}{25} & \frac{4209}{7225} & \frac{-741}{7225} \\
\frac{60}{289} & \frac{21}{289} & \frac{2421}{7225} & \frac{-1554}{7225} & \frac{54}{7225} & \frac{-921}{7225} & \frac{21}{289} & \frac{3}{25} & \frac{-741}{7225} & \frac{4209}{7225}
\end{bmatrix} \tag{S12}
$$

## Eq. (44) In Terms of Computable Quantities

We express the matrix elements pertinent to evaluating Eq. (44) in terms of readily computable quantities. We write the following matrix elements,

$$
\mu_{ab} = \langle \Psi_0 | \hat{\mathcal{H}} \left| \Phi_{(ab)} \right\rangle = -\sqrt{3}\sigma_{ab;st_2;st_3}, \tag{S13}
$$

and

$$
\kappa_{Ka;b} = \sqrt{6} \left\langle \Psi_{[K]_1[a]_2[b]_3} \right| \hat{\mathcal{H}} \left| \Phi_{(Ka)} \right\rangle = \sqrt{2} \left( \sigma_{ab;t_2t_1;t_3s} - \sigma_{Kb;t_1t_3;t_3s} \right) \tag{S14}
$$

where we used the fact that Hamiltonian commutes with a singlet-projection operator and both bra and ket states are singlets and

$$
\left\langle \Psi_{[K]_1[a]_2[b]_3} \right| \hat{\mathcal{H}} \left| \Phi_{(Ka)} \right\rangle = \langle 0 | \hat{g}_{t_1,K} \hat{g}_{t_2,a} \hat{g}_{t_3,b} \hat{\mathcal{H}} \hat{d}^{\dagger}_{s2,Ka} \hat{g}^{\dagger}_{s,b} |0\rangle = \frac{1}{\sqrt{3}} \left( \sigma_{ab;t_2t_1;t_3s} - \sigma_{Kb;t_1t_3;t_3s} \right). \tag{S15}
$$

Similarly,

$$\left\langle \Psi_{(KLa)} \right| \hat{\mathcal{H}} \left| \Psi_{(KLa)} \right\rangle = \sqrt{6} \left\langle \Psi_{(KLa)} \right| \hat{\mathcal{H}} \left| \Psi_{[K]_1[L]_2[a]_3} \right\rangle \tag{S16}$$

$$= -\sigma_{KL;t_2t_1;t_1t_2} - \sigma_{Ka;t_3t_1;t_1t_3} + \left\langle \Psi_{[K]_1[L]_2[a]_3} \right| \hat{\mathcal{H}} \left| \Psi_{[K]_1[L]_2[a]_3} \right\rangle \tag{S17}$$

Using this, we write $\omega_{KLa}$ in terms of computable quantities:

$$\begin{aligned}
\omega_{KLa} &= \left\langle \Psi_{(KLa)} \right| \hat{\mathcal{H}} \left| \Psi_{(KLa)} \right\rangle - \left\langle \Psi_0 \right| \hat{\mathcal{H}} \left| \Psi_0 \right\rangle \\
&= -\sigma_{KL;t_2t_1;t_1t_2} - \sigma_{Ka;t_3t_1;t_1t_3} \\
&+ \eta_{K;t_1t_1} + \eta_{L;t_2t_2} + \eta_{a;t_3t_3} - \eta_{K;ss} - \eta_{L;ss} - \eta_{a;ss} \\
&+ \rho_{K;t_1;t_1} + \rho_{L;t_2;t_2} + \rho_{a;t_3;t_3} - \rho_{K;s;s} - \rho_{L;s;s} - \rho_{a;s;s} \\
&+ \sigma_{KL;t_1t_1;t_2t_2} + \sigma_{Ka;t_1t_1;t_3t_3} + \sigma_{La;t_2t_2;t_3t_3} - \sigma_{KL;ss;ss} - \sigma_{Ka;ss;ss} - \sigma_{La;ss;ss} \\
&+ \sum_{b \notin \{K,L,a\}} \left( \sigma_{Kb;t_1t_1;ss} + \sigma_{Lb;t_2t_2;ss} + \sigma_{ab;t_3t_3;ss} - \sigma_{Kb;ss;ss} - \sigma_{Lb;ss;ss} - \sigma_{ab;ss;ss} \right)
\end{aligned} \tag{S18}$$

# CCVB+i3 Jacobian

We derive the CCVB+i3 Jacobian which is used in amplitude solvers. The Jacobian reads

$$(J)_{Ka,Mc} = \frac{\partial \Omega_{Ka}}{\partial t_{Mc}} = \frac{\partial R_{Ka}}{\partial t_{Mc}} + \sum_{b \notin \{K,a\}} \frac{\partial t_{Kab}}{\partial t_{Mc}} \kappa_{Ka;b} \tag{S19}$$

where

$$\begin{aligned}
\frac{\partial R_{Ka}}{\partial t_{Mc}} &= \left[ \omega_{Ka} - 2t_{Ka}\mu_{Ka} - \sum_{b \notin \{K,a\}} \left( t_{Kb}\mu_{Kb} + t_{ab}\mu_{ab} \right) \right] \delta_{Ka,Mc} \\
&+ \sum_{b \notin \{K,a\}} \left[ (\kappa_{Kb} - t_{Ka}\mu_{ab})\delta_{ab,Mc} + (\kappa_{ab} - t_{Ka}\mu_{Kb})\delta_{Kb,Mc} \right]
\end{aligned} \tag{S20}$$

and using Eq. (44) we obtain

$$\frac{\partial t_{Kab}}{\partial t_{Mc}} = \delta_{Ka,Mc}\left[\frac{\kappa_{Ka;b}}{\Delta_{Kab}} - \frac{\mu_{Ka}}{\Delta_{Kab}}t_{Kab}\right] + \delta_{Kb,Mc}\left[-\frac{\kappa_{Kb;a}}{\Delta_{Kab}} - \frac{\mu_{Ka}}{\Delta_{Kab}}t_{Kab}\right]$$
$$+ \delta_{Lb,Mc}\left[\frac{\kappa_{ab;K}}{\Delta_{Kab}} - \frac{\mu_{ab}}{\Delta_{Kab}}t_{Kab}\right] \tag{S21}$$

where

$$\Delta_{Kab} = (t_{Ka}\mu_{Ka} + t_{Kb}\mu_{Kb} + t_{ab}\mu_{ab}) - \omega_{Kab} \tag{S22}$$

## CCVB+i3 Lagrangian and Its Derivatives

We derive derivatives of the CCVB+i3 Lagrangian defined in Eq. (48) and write them in terms of computable quantities. From

$$\frac{\partial \mathcal{L}}{\partial t_{Ka}} = 0, \tag{S23}$$

we obtain

$$0 = \frac{\partial E}{\partial t_{Ka}} + \sum_{M<b} \lambda_{Mb}\frac{\partial R_{Mb}}{\partial t_{Ka}} + \sum_{b\notin\{K,a\}} \lambda_{Kab}\left(\kappa_{Ka;b} - t_{Kab}\mu_{Ka}\right). \tag{S24}$$

We already have $\frac{\partial R_{Mb}}{\partial t_{Ka}}$ from Eq. (S20) and we have

$$\frac{\partial E}{\partial t_{Ka}} = \mu_{Ka} \tag{S25}$$

For the gradient of $\mathcal{L}$ with respect to some parameters $\mathbf{X}$ (either $\Theta$ or $\Delta$), most terms are already discussed in ref. 61 and we discuss the 3P specific terms. First, consider

$$\frac{\partial}{\partial \mathbf{X}}\sum_{K<a}\sum_{b\notin\{K,a\}} t_{Kab}\kappa_{Ka;b} = \sqrt{2}\sum_{K<a}\sum_{b\notin\{K,a\}} t_{Kab}\frac{\partial}{\partial \mathbf{X}}\left(\sigma_{ab;t_2t_1;t_3s} - \sigma_{Kb;t_1t_3;t_3s}\right) \tag{S26}$$

$$= \sqrt{2}\sum_{K<a}\sum_{b\notin\{K,a\}} t_{Kab}\left(\sigma^{\mathbf{X}}_{ab;t_2t_1;t_3s} - \sigma^{\mathbf{X}}_{Kb;t_1t_3;t_3s}\right) \tag{S27}$$

Here, we learned that

$$\kappa^{\mathbf{X}}_{Ka;b} = \sqrt{2}\left(\sigma^{\mathbf{X}}_{ab;t_2t_1;t_3s} - \sigma^{\mathbf{X}}_{Kb;t_1t_3;t_3s}\right) \tag{S28}$$

The derivatives of $\sigma$'s with respect to $\Theta$ and $\Delta$ are available in ref. 61. The same applies to the diagonal elements of Hessian. Similarly, the last term in Eq. (48) follows

$$\sum_{K<L<a} \lambda_{KLa} \frac{\partial^{(3)}\Omega_{KLa}}{\partial \mathbf{X}} = \sum_{K<L<a} \lambda_{KLa}(t_{KL}\kappa^{\mathbf{X}}_{KL;a} - t_{Ka}\kappa^{\mathbf{X}}_{Ka;L} + t_{La}\kappa^{\mathbf{X}}_{La;K} - t_{KLa}(-\omega^{\mathbf{X}}_{KLa} + t_{KL}\mu^{\mathbf{X}}_{KL} + t_{Ka}\mu^{\mathbf{X}}_{Ka} + t_{La}\mu^{\mathbf{X}}_{La})) \tag{S29}$$

Based on Eq. (S18), we can compute $\omega^{\mathbf{X}}_{KLa}$ in terms of other more fundamental quantities discussed in ref. 61. For $\kappa$ derivatives, we apply Eq. (S28). $\mu$ derivatives are available in ref. 61. The same applies to the diagonal elements of Hessian.
